# Supplementary material for: Notes on kAExp(pol) problems for deterministic machines
Source: arXiv:2110.05630 source file (2021-10-11)
Supplement: Supplementary file 1 [file appendix.tex]

\input{appendix-on-tetration}
\input{appendix-alternating-turing-machines}
